# Supplementary material for: Generating graph states with a single quantum emitter and the minimum number of fusions
Source: arXiv:2412.04587 source file (2025-04-09)
Supplement: Supplementary file 1 [file supplemental_material.pdf]

# Supplemental material for "Generating graph states with a single quantum emitter and the minimum number of fusions"

Matthias C. Löbl,[1] Love A. Pettersson,[1] Andrew Jena,[2] Luca Dellantonio,[3] Stefano Paesani,[1,4] and Anders S. Sørensen[1]

[1] *Center for Hybrid Quantum Networks (Hy-Q), The Niels Bohr Institute, University of Copenhagen, Blegdamsvej 17, DK-2100 Copenhagen Ø, Denmark*
[2] *Department of Combinatorics and Optimization, University of Waterloo and Institute for Quantum Computing, University of Waterloo*
[3] *Department of Physics and Astronomy, University of Exeter, Stocker Road, Exeter EX4 4QL, United Kingdom*
[4] *NNF Quantum Computing Programme, Niels Bohr Institute, University of Copenhagen, Blegdamsvej 17, DK-2100 Copenhagen Ø, Denmark.*

## I. COMPARISON TO DETERMINISTIC GRAPH STATE GENERATION

In this section, we give an overview of the resources required to construct graph states of up to eight qubits. In Figs. 1 and2, we show the number of fusions required to build graph states when using a single quantum emitter. We furthermore compare the number of fusions to the number of quantum emitters required to generate the graph state deterministically [1].

[1] Bikun Li, Sophia E. Economou, and Edwin Barnes. "Photonic resource state generation from a minimal number of quantum emitters". Npj Quantum Inf. **8**, 11 (2022).

[2] M. Hein, J. Eisert, and H. J. Briegel. "Multiparty entanglement in graph states". Phys. Rev. A **69**, 062311 (2004).

[3] Adán Cabello, Antonio J López-Tarrida, Pilar Moreno, and José R. Portillo. "Entanglement in eight-qubit graph states". Physics Letters A **373**, 2219–2225 (2009).

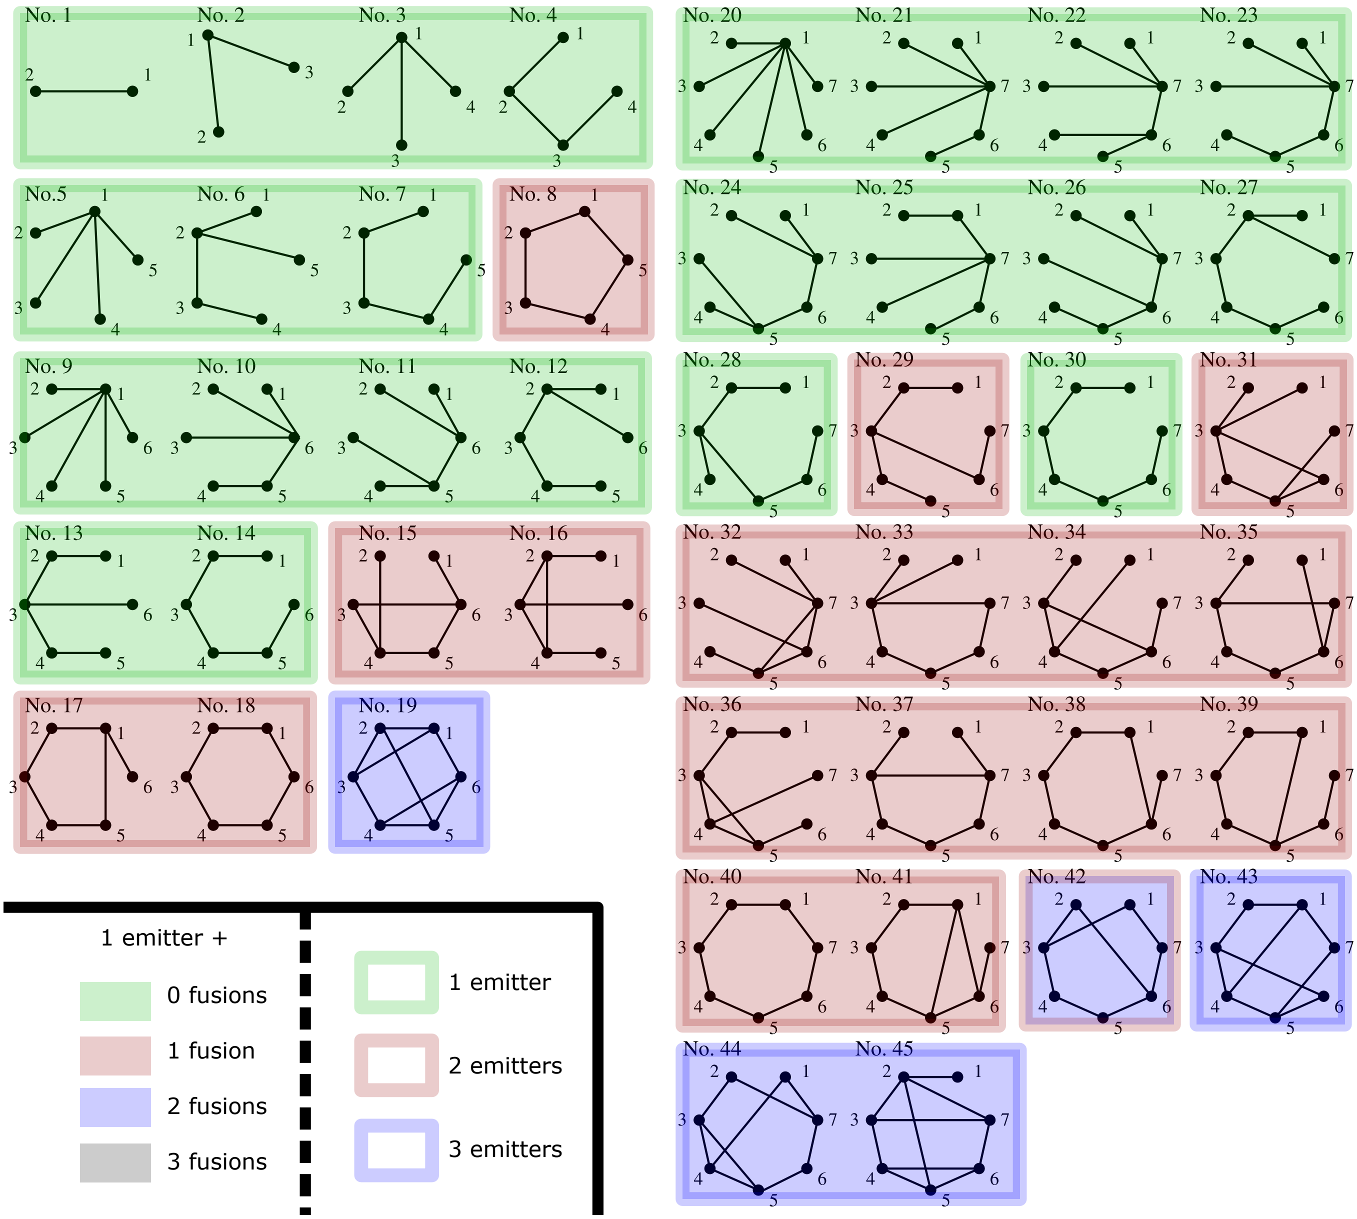


Figure 1. One representative graph state per graph orbit for graph states with up to seven qubits (adapted from Ref. [2]). The number of fusions required to generate the corresponding state using only a single quantum emitter is illustrated by the face color of every square box. The number of emitters required to generate the graph state deterministically is illustrated by the frame color of every box. This number is obtained by computing the height function introduced in Ref. [1]. Apart from orbit no. 42, the inequality in Eq. (2) from the main text is saturated with an equal sign.

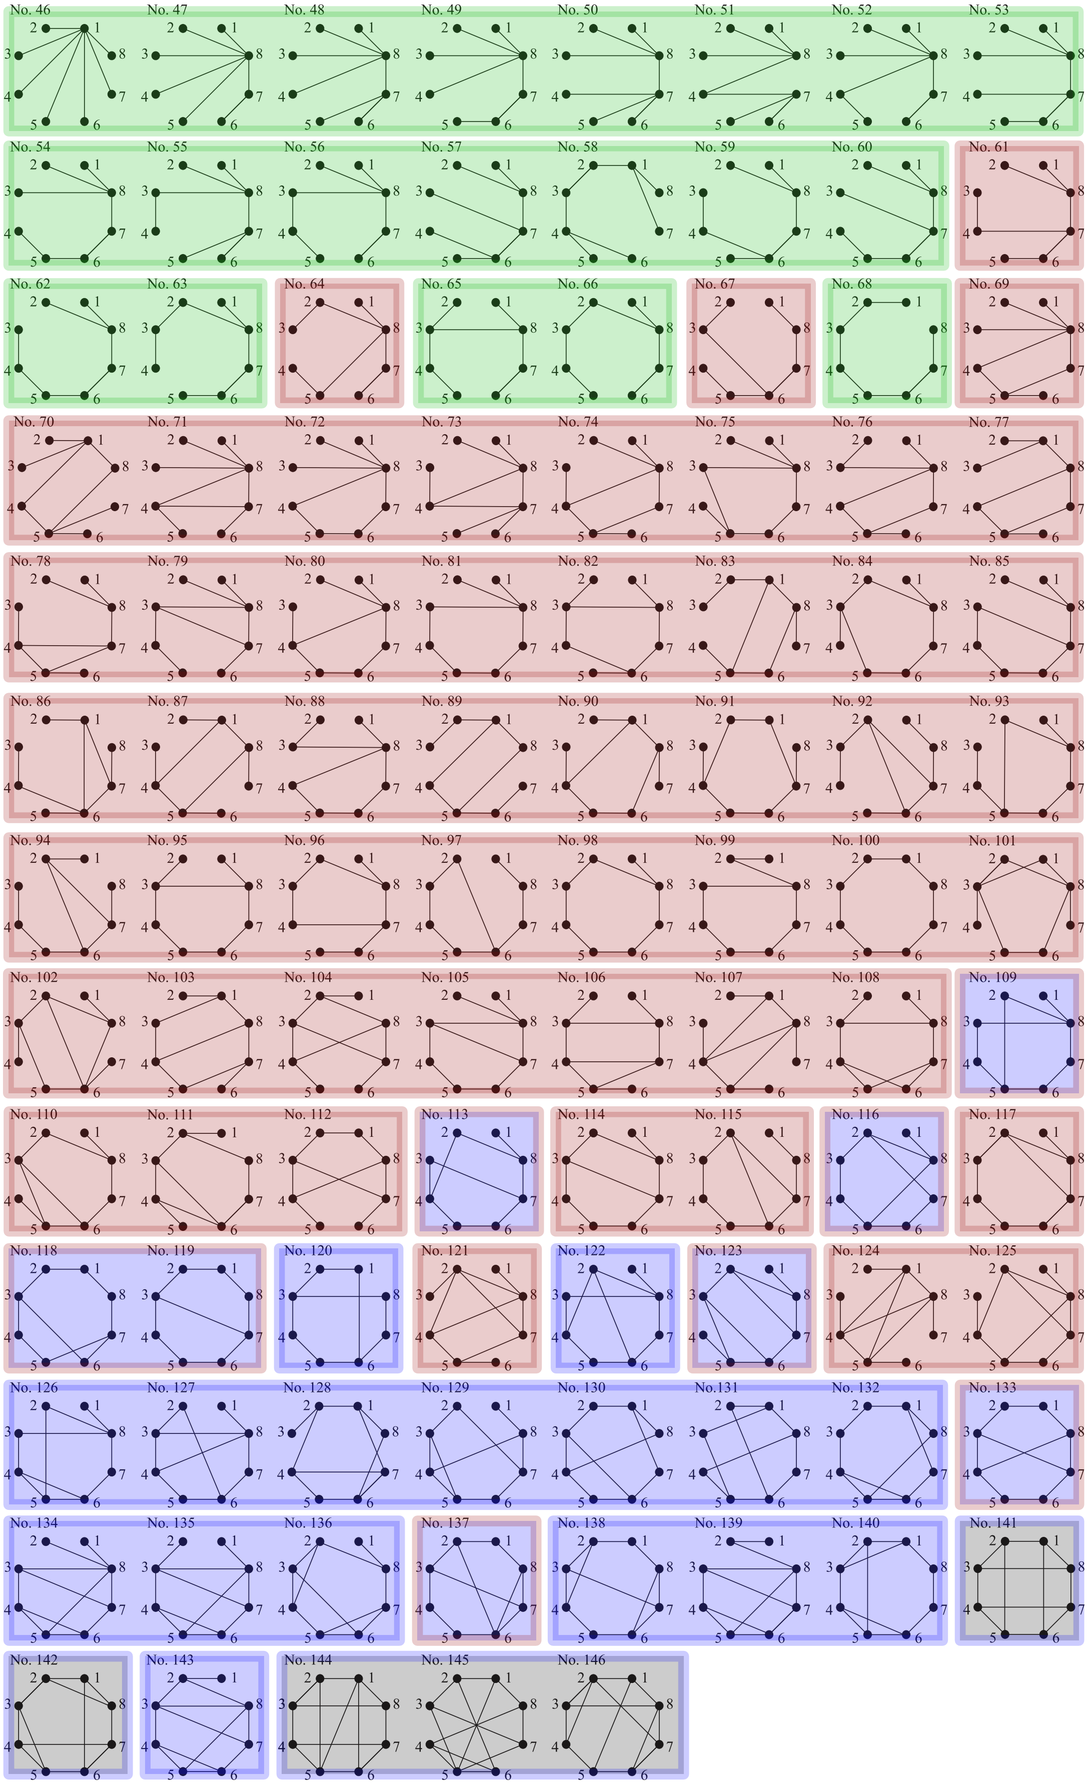


Figure 2. One representative graph state per graph orbit for graph states with eight qubits (adapted from Ref. [3]). The number of fusions required to generate the corresponding state using only a single quantum emitter is illustrated by the different colors and compared to the number of static qubits required to generate the graph state deterministically (see previous figure for the color legend). The inequality in Eq. (2) from the main text is not saturated for 13 out of the 101 graph orbits.
